# Supplementary material for: Instance-wise Graph-based Framework for Multivariate Time Series Forecasting
Source: arXiv:2109.06489 source file (2021-09-14)
Supplement: Supplementary file 1 [file appendix.tex]

\begin{comment}
\appendix
\section{Datasets}
\subsection{Time Series Forecasting}
\label{subsec:timeseries_data}
\begin{itemize}
	\item Traffic: the traffic dataset from the California Department of Transportation contains road occupancy rates measured by 862 sensors in San Francisco Bay area freeways during 2015 and 2016.
	%	\item Solar-Energy: the solar-energy dataset from the National Renewable Energy Laboratory contains the solar power output collected from 137 PV plants in Alabama State in 2007.
	\item Electricity:  the electricity dataset from the UCI Machine Learning Repository contains electricity consumption for 321 clients from 2012 to 2014.
	\item Exchange-Rate: the exchange-rate dataset contains the daily exchange rates of eight foreign countries including Australia, British, Canada, Switzerland, China, Japan, New Zealand, and Singapore ranging from 1990 to 2016.
\end{itemize}
\subsection{Stock Trend Forecasting}


\section{Details of Compared Methods}
\subsection{Compared Methods on Stock Trend Forecasting}
\label{subsec:stock_method}
We compare our proposed HIST framework with the following stock trend forecasting methods:
\begin{itemize}[leftmargin=1.5em]
	\item \textbf{ARIMA}~\cite{brown2004smoothing}: Autoregressive Integrated Moving Average uses historical stock trend series to forecast the stock future trend.
	\item \textbf{MLP}: A $3$-layers multi-layer perceptron (MLP) with the number of units on each layer is $512$.
	\item \textbf{LSTM}~\cite{hochreiter1997long}: A $2$-layer Long Short-Term Memory (LSTM) network with the number of hidden units is $128$.
	\item \textbf{GRU}~\cite{chung2014empirical}: A $2$-layer Gated Recurrent Unit (GRU) network that has $128$ units in the hidden states.
	\item \textbf{RSR\_E}~\cite{feng2019temporal}: RSR\_E can model the cross-stock impact of different stocks' features by leveraging a variant of graph convolutional networks~\cite{kipf2017semi}. We followed the same experimental setting of RSR\_E and utilized the industrial relations of stocks, which are also used in the experiment of RSR\_E.
	\item \textbf{Adv-ALSTM}~\cite{feng2019enhancing}: A stock prediction framework that leverages the adversarial training to simulate the stochasticity during model training.
\end{itemize}



\subsection{Evaluation Metric on Stock Trend Forecasting}
\label{subsec:stock_metric}
\begin{itemize}[leftmargin=1.5em]
	\item \textbf{Cumulative Return (CR)} is a the aggregate amount that the investment has gained or lost over time, and the cumulative return is calculated by: ${\rm CR} = \dfrac{\rm current\ capital - initial\ captial}{\rm initial\ captial}$.
	\item \textbf{Sharpe Ratio (SHR)} is a measurement of  an investment compared to a risk-free asset, after adjusting for its risk. It is defined as: ${\rm SHR} = \dfrac{\rm E[R_a - R_b]}{\sqrt{\rm var[R_a - R_b]}}$, where $R_a$ is the return of given portfolio and $R_b$ denotes the risk-free return. $\rm E[\cdot]$ is the expected value, and $\rm var[\cdot]$ is the variance.
\end{itemize}


\section{Application to Stock Trend Forecasting}
\label{sec:experiment_stock}





\subsection{Task Description}

\subsection{Background}
In recent years, stock trend forecasting has attracted soaring attention because it is vital in stock investment. 
%This section will introduce two representative categories of stock trend forecasting methods: technical analysis and event-driven stock trend forecasting methods. 
The technical analysis~\cite{edwards2018technical} predicts the stock trend based on the historical time-series of market data, such as trading price and volume. 
It aims to discover the trading patterns that we can leverage for future predictions.
We can further divide the technical analysis methods into the \textbf{Single-stock Methods} and the \textbf{Cross-stock Methods}. 
The single-stock methods only use each stock's information to forecast the stock trend, and the cross-stock methods consider the cross-stock relationships between stocks when they forecast the stock price trend.
\paragraph{Single-stock methods}
For the single-stock methods, Autoregressive (AR)~\cite{li2016stock}, and ARIMA~\cite{ariyo2014stock} models are the most widely used model in this direction, which are both for linear and stationary time-series. However, the non-linear and non-stationary nature of stock prices limits the applicability of AR and ARIMA models. 
Some studies~\cite{ticknor2013bayesian,patel2015predicting} attempted to apply deep neural networks to catch the market trend's intricate patterns with the recent rapid development of deep learning. 
To further model the long-term dependency in time series, recurrent neural networks (RNN), especially Long Short-Term Memory (LSTM) network~\cite{hochreiter1997long}, had also been employed in financial predition~\cite{rather2015recurrent,gao2016stock,akita2016deep,bao2017deep}. Specifically,~\cite{zhang2017stock} proposed a new State Frequency Memory (SFM) recurrent network to discover the multi-frequency trading patterns for stock price movement prediction;~\cite{li2019multi} presented a multi-task recurrent neural network with high-order Markov random fields (MRFs) to predict stock price movement direction;~\cite{feng2019enhancing} leveraged adversarial training to simulate the stochasticity during model training. However, each stock is not isolated; the single-stock methods can not utilize the cross-stock interactions between stocks to capture more information for stock trend forecasting.
\paragraph{Cross-stock Methods}
To mine the cross-stock shared information and improve the stock trend forecasting performance, many cross-stock methods~\cite{chen2018incorporating,feng2019temporal,kim2019hats,matsunaga2019exploring} leveraged the Graph Neural Networks~\cite{kipf2017semi,velickovic2018graph} to capture the relationships between different stocks. The~\cite{chen2018incorporating} and~\cite{feng2019temporal} utilize the graph convolutional networks (GCN) to capture the stocks' shareholder relations and industry relations, respectively. The~\cite{kim2019hats} propose a hierarchical attention network for stock prediction (HATS), which uses relational data for stock market prediction.
However, these existing cross-stock methods can not correctly utilize the shared information of predefined concepts because they use stationary relations to aggregate information and neglect dynamic relevance between the stocks and predefined concepts.
Additionally, they also overlook the invaluable shared information of hidden concepts, limiting their stock trend forecasting performance. 


\begin{table}
	\begin{center}
		%		\resizebox{\columnwidth}{!}{%
		\begin{tabular}{l|rrrr} 
			\toprule
			Datasets 		& \# Training		& \# Validation	& \#Test \\
			\midrule
			\midrule
			CSI 100 		& 17,544 	& 862 	& 1 hour 	\\
			CSI 300 	& 26,304 	& 321 	& 1 hour 	\\
			\bottomrule
		\end{tabular}%}
	\end{center}
	\caption{Statistics of Stock Trend Forecasting Datasets.}
	\label{table:stock-dataset}
\end{table}
\subsection{Settings}
\paragraph{Datasets} 
We evaluate our HIST framework on the stocks of two popular and representative stock indexes: CSI 300 and CSI 500. CSI 300 index consists of the $300$ largest and the most liquid stocks; CSI 500 index comprises the largest remaining $500$ stocks after excluding the CSI 300 Index constituents. The CSI 300 and CSI 500 indexes reflect the market's overall performance and small-mid cap stocks.

\begin{table*}[t]
	\label{tab:results}
	\centering
	\resizebox{1\textwidth}{!}{
		\begin{threeparttable}
			\begin{tabular}{l|c|c|cccc|c|c|cccc}
				\toprule
				\multirow{3}{*}{Methods} & \multicolumn{6}{c|}{CSI 100} & \multicolumn{6}{c}{CSI 300} \\
				\cmidrule(lr){2-13} & \multirow{2}{*}{IC} &\multirow{2}{*}{Rank IC} & \multicolumn{4}{c|}{Precision@N ($\uparrow$)}& \multirow{2}{*}{IC} &\multirow{2}{*}{Rank IC} & \multicolumn{4}{c}{Precision@N ($\uparrow$)} \\
				\cmidrule(lr){4-7}
				\cmidrule(lr){10-13}
				&  ($\uparrow$)& ($\uparrow$) & 3 & 5 & 10& 30& ($\uparrow$) & ($\uparrow$)& 3 & 5 & 10& 30\\
				\midrule
				\midrule 
				MLP&0.0666&0.0647&56.12\% & 55.82\% & 55.68\%& 53.58\%& 0.0832& 0.0803& 58.29\% & 57.23\% & 56.65\%& 55.76\%\\ 
				LSTM & 0.0972& 0.0909& 60.59\% & 59.26\% & 57.82\%& 54.60\%& 0.1084& 0.1035& 60.21\% & 60.14\% & 59.36\%& 57.52\%\\ 
				SFM& 0.0787& 0.0726& 57.88\% & 57.08\% & 55.76\%& 53.84\%& 0.1074& 0.1014& 61.17\% & 59.90\% & 58.61\%& 57.71\%\\ 
				GRU & 0.1037& 0.0968& 59.32\% & 58.74\% & 58.24\%& 55.09\%& 0.1153& 0.1097& 60.18\% & 60.06\% & 58.91\%& 57.63\%\\ 
				GATs& 0.0981&0.0947& 58.43\%& 58.46\% & 57.48\%&55.09\% & 0.1097& 0.1048& 60.38\% & 58.95\% & 58.31\%& 57.42\%\\ 
				ALSTM&0.1006 &0.0961&60.14\% & 59.23\% &57.71\% & 54.75\%&0.1133& 0.1082& 60.21\% & 59.90\% & 58.97\%& 57.77\%\\ 
				\midrule
				\textbf{Ours}	& && &  & & &$\textbf{0.1233}$& $\textbf{0.1169}$& $\textbf{62.10\%}$ & $\textbf{61.50\%}$ & $\textbf{60.39\%}$& $\textbf{58.70\%}$\\ 
				\bottomrule
			\end{tabular}
		\end{threeparttable}
	}
	\caption{The main results on CSI 100 and CSI 300.}
\end{table*}
\paragraph{Stock Price and Volume Data}
We collect the daily stock price and volume data of the stocks in CSI 300 and CSI 500 indexes from Jan. 1, 2007, to Dec. 31, 2019\footnote{We collect daily stock price and volume data from \url{http://xueqiu.com}.}, and split them by time to a training period from 2007 to 2014, a validation period from 2015 to 2016, and a test period from 2017 to 2019. There are $6$ stock price and volume data on each day, which are \textit{opening price}, \textit{closing price}, \textit{highest price}, \textit{lowest price}, \textit{volume weighted average price} (VWAP) and \textit{trading volume}. 
For each stock on date $t$, we look back $30$ days to construct $180$-dimensional historical stock price and volume data as stock features. For these $180$-dimensional stock features, we divide all of the price indicators by the closing price of date $t$ to get the relative change and divide the volume indicators by the volume of date $t$ to get relative transaction volume. We use the stock trend defined on Equation~\ref{eq:stock-trend} as the label, and we apply normalization on the labels of the same date.
\subsubsection{Evaluation Metrics}
%To evaluate the results of stock trend forecasting, we firstly use three standard regression evaluation metrics, which are \textbf{Root Mean Squared Error (RMSE)}, \textbf{Mean Absolute Error (MAE)} and \textbf{Median Absolute Error (MedAE)}.
%Specifically, RMSE is defined by: $\mathrm{RMSE}(y, \hat{y}) = \sqrt{\frac{1}{n} \sum_{i=1}^n (y_i - \hat{y}_i)^2}$;
%MAE is the mean value of absolute error between labels and predictions: $\mathrm{MAE}(y, \hat{y}) = \frac{1}{n} \sum_{i=1}^n |y_i - \hat{y}_i|$;
%MedAE is the median of absolute error between labels and predictions: $\mathrm{MedAE}(y, \hat{y}) = \mathrm{median}(|y_1-\hat{y}_1|, ..., |y_n - \hat{y}_n|)$. 
%$R^2$ is calculated by: $R^2(y, \hat{y}) =1-\dfrac{\sum_i{\left(y_i - \hat{y_i}\right)}}{\sum_i{\left(y_i - \bar{y}\right)}}$, where $\bar{y}$ is the mean of labels $y$: $\bar{y}=\frac{1}{n} \sum_{i=1}^n y_i$.
To evaluate the results of stock trend forecasting, we firstly use two standard regression evaluation metrics, which are \textbf{Mean Squared Error (MSE)} and \textbf{Mean Absolute Error (MAE)}.
Specifically, given the labels $y$ and the predictions $\hat{y}$, MSE is calculated by: $\mathrm{MSE}(y, \hat{y}) = \frac{1}{n} \sum_{i=1}^n (y_i - \hat{y}_i)^2$;
MAE is the mean value of absolute error between labels and predictions: $\mathrm{MAE}(y, \hat{y}) = \frac{1}{n} \sum_{i=1}^n |y_i - \hat{y}_i|$.
Moreover, we also use two widely used indicators in the quantitative investment domain: the \textbf{Information Coefficient (IC)} and \textbf{Rank IC}~\cite{li2019individualized}.
The IC is the Pearson correlation coefficient~\cite{benesty2009pearson} between the labels and predictions. 
The Rank IC is the Spearman's rank correlation coefficient, calculated by: $\mathrm{Rank\ IC}(y^t, \hat{y}^t) = \mathrm{corr}(rank_{y}^t, rank_{\hat{y}}^t)$, where $\mathrm{corr}(\cdot)$ is the Pearson correlation coefficient. 
We sort the stock trend labels and predictions of all stocks on each day from high to low and acquire the ranks $rank_{y}^t$ and $rank_{\hat{y}}^t$ of each stock's labels and predictions on the date $t$. 
We use the average IC and Rank IC of each day to evaluate the results of stock trend forecasting. 
To eliminate the fluctuations caused by different initialization, we repeat the testing procedure ten times for all the results and report the average value.


\begin{figure*}[t]
	\centering
	\subfigure[The Cumulative Return on CSI 300.]{\includegraphics[width=0.8\columnwidth]{figure/csi300_cumulative_return}}
	\hspace{.5in}
	\subfigure[The Cumulative Return on CSI 500.]{\includegraphics[width=0.8\columnwidth]{figure/csi500_cumulative_return}}
	%	\vspace{-.1in}
	\caption{The results of Cumulative Return.}
	%	\vspace{-.1in}
	\label{fig:return}
\end{figure*} 
\subsubsection{Hyper-parameters Setting}
The dimension of stock features $l$ is $180$. In the stock features encoder, the number of units $d$ in the hidden state of GRU is $128$. In the three modules of our framework, the number of units in the fully-connected layers is also $128$, and the learning rate of our HIST framework is $2 \times 10^{-4}$.

\subsubsection{Compared Methods} 
We compared our method with the some stock trend forecasting method, including MLP,  LSTM~\cite{hochreiter1997long}, GRU~\cite{chung2014empirical}, RSR\_E~\cite{feng2019temporal}, Adv-ALSTM~\cite{feng2019enhancing}. The details of these method are described in Appendix~\ref{subsec:stock_method}.





\subsection{Results and Analysis}
\paragraph{Main Results}
Table $1$ shows the experimental results of HIST and some other compared methods on the stocks of CSI 300 and CSI 500 indexes. Our HIST framework achieves the lowest MSE, MAE, and the highest IC, Rank IC compared with the baselines. From Table $1$ we can find that the traditional ARIMA model and the simple MLP model have a weak performance, and some latest methods such as the RSR\_E and Adv-ALSTM have relatively better results. However, our proposed HIST framework is not only better than the LSTM and GRU model but also can achieve a better result than the latest stock trend forecasting methods like RSR\_E and Adv-ALSTM. Although the RSR\_E can also capture the cross-stock connections, the cross-stock relations in RSR\_E are stationary. 
Our proposed HIST can model the dynamic relevance degree between stocks and concepts, and thus capture the temporal and complicated cross-stock relations between stocks. 
Moreover, our method can also mine the shared information of hidden concepts, so our HIST model outperforms existing graph neural networks based cross-stock technical analysis methods, such as the RER\_E.



\begin{figure}[t]
	\centering
	\includegraphics[width=1\columnwidth]{figure/legend}
	\vspace{.05in}
	\subfigure[Sharpe Ratio on CSI 300.]{\includegraphics[width=0.48\columnwidth]{figure/csi300_sharpe}}
	\hspace{.05in}
	\subfigure[Sharpe Ratio on CSI 500.]{\includegraphics[width=0.48\columnwidth]{figure/csi500_sharpe}}
	%	\vspace{-.1in}
	\caption{The results of Sharpe Ration.}
	%	\vspace{-.1in}
	\label{fig:sharpe}
\end{figure} 

\subsubsection{Investment Simulation}
To further evaluate our proposed HIST framework's effectiveness, we utilize an investment strategy to simulate the investment in the year 2019. Specifically, we rank the stocks on date $t$ from high to low according to the stock trend's prediction, then select the top $k$ stocks to evenly invest and sell the last $k'$ stocks among the currently held stocks. To approximate real-world trading, we assume the initial account capital is $1 e^8$, and we consider a transaction cost of $0.05\%$ for the buying shares and $0.15\%$ for the selling shares. We use two financial metrics to evaluate the investment simulation result, which is the Cumulative Return and Sharpe Ratio~\cite{sharpe1966mutual}:

To find the best selection of the number of stocks we choose to buy $k$ and the number of stocks we sell $k'$, we conduct a grid search to find the best value that maximizes the investment return on the validation set. We tune the $k\in \{10, 20, 30, 40, 50\}$ and $k'\in \{1, 3, 5, 7, 9\}$,  and we find that we can achieve the highest return when $k$ is 10 and $k'$ is $5$ in CSI 300, and $k$ is 40 and $k'$ is $5$ in CSI 500.
Figure~\ref{fig:return} shows the simulation results of the Cumulative Return on CSI 300 and CSI 500 indexes, which illustrates that our HIST framework can gain the highest Cumulative Return.
Figure~\ref{fig:sharpe} is the results of the Sharpe Ratio, and our HIST framework also can achieve the highest Sharpe Ratio compared with the baselines.
From Figure~\ref{fig:return} and Figure~\ref{fig:sharpe} we know that our HIST framework is not only outperforming some basic MLP, LSTM, and GRU models but also better than some latest state-of-the-art methods, such as the RSR\_E and Adv-ALSTM.
These results of investment simulation further confirm the effectiveness of our HIST framework.
\end{comment}
